# Supplementary material for: Learning an Efficient Optimizer via Hybrid-Policy Sub-Trajectory Balance
Source: arXiv:2511.00543 source file (2025-11-01)
Supplement: Supplementary file 1 [file appendix.tex]

\clearpage
\appendix
\onecolumn
\setcounter{page}{1}
\setcounter{theorem}{0}
\setcounter{assumption}{0}
\setcounter{equation}{0}
\setcounter{section}{0}

\section{Proofs of Theorem 1 and Theorem 2}\label{app:prof12}
\begin{theorem}\label{thm:sub-tra}
Suppose that $\mathcal{L}_{hy}^{sub} = 0$.
Then, the expected cumulative probability of the sub-inference trajectories \(\tau^{m':n'}_{on}=\{s_{m'},\cdots, s_{n'}\}\) satisfies
\[
\underset{{\tau\in\mathcal{T}_{m':n'}}}{E}\prod_{t=m'}^{n'-1}P^F_{\phi}(s_{t+1}\mid s_t) \;\propto\; R_{n}(s_{n'}).
\]
\end{theorem}

\begin{proof}
Since \(E(\mathcal{L}_{hy}^{sub})=0\), for any fixed indices \(m<n\), each online sub-trajectory \(\tau^{m':n'}_{on}=\{s_{m'}\to\cdots\to s_{n'}\}\) satisfies
\[
  \log C_{\phi}(s_{m'})\,R_n(s_{m'})
  + \sum_{t=m'}^{n'-1}\log P^F_{\phi}(s_{t+1}\mid s_t)
  = \log C_{\phi}(s_{n'})\,R_n(s_{n'})
  + \sum_{t=m'}^{n'-1}\log P^B_{\phi}(s_t\mid s_{t+1}).
\]
Exponentiating both sides gives
\[
  C_{\phi}(s_{m'})\,R_n(s_{m'})\;\prod_{t=m'}^{n'-1}P^F_{\phi}(s_{t+1}\mid s_t)
  = C_{\phi}(s_{n'})\,R_n(s_{n'})\;\prod_{t=m'}^{n'-1}P^B_{\phi}(s_t\mid s_{t+1}).
\]
Summing over \(\mathcal{T}_{m\to n}\) and using the fact that
\(\sum_{\tau\in\mathcal{T}_{m'\to n'}}\prod_{t=m'}^{n'-1}P^B_{\phi}(s_t\mid s_{t+1})=1\)
(see Equation 18 in the proof of Trajectory Balance~\cite{TB} for details), we obtain
\[
  C_{\phi}(s_{m'})\,R_n(s_{m'})
  \sum_{\tau\in\mathcal{T}_{m'\to n'}}\prod_{t=m'}^{n'-1}P^F_{\phi}(s_{t+1}\mid s_t)
  = C_{\phi}(s_{n'})\,R_n(s_{n'}).
\]
Rearranging yields
\[
  \sum_{\tau\in\mathcal{T}_{m'\to n'}}\prod_{t=m'}^{n'-1}P^F_{\phi}(s_{t+1}\mid s_t)
  = \frac{C_{\phi}(s_{n'})}{C_{\phi}(s_{m'})\,R_n(s_{m'})}\,R_n(s_{n'}),
\]
As a result, we have
$$
E_{\tau\in\mathcal{T}_{m'\to n'}}\prod_{t=m'}^{n'-1}P^F_{\phi}(s_{t+1}\mid s_t) \;\propto\; R_{n}(s_{n'}).
$$

\end{proof}

\begin{theorem}\label{thm:full-tra}
Suppose that $\mathcal{L}_{hy}^{sub} = 0$.
Then, the expected cumulative probability of the full inference trajectory $\tau^{0:N}_{on}=\{s_0,...,s_N\}$ satisfies
\[
\underset{{\tau\in\mathcal{T}_{0:N}}}{E}\prod_{t=1}^{N-1} P^F_{\phi}(s_{t+1}\mid s_{t}) \;\propto\; R_{T}(s_N).
\]
\end{theorem}

\begin{proof}
Fix a divisor \(d\) of \(N\), and for each \(i \in \{0,1,\dots,\tfrac{N}{d}-1\}\), we define the segmentwise residual\footnote{For simplicity, we omit the subscripts in \(C_{\phi}\), \(P_{\phi}^F\), and \(P_{\phi}^B\), as well as the argument \((s_{t+1}\mid s_t)\) in \(P^F_{\phi}(\cdot)\) and \(P^B_{\phi}(\cdot)\)}
\[
g_i \;=\;
\log C(s_{i d})\,R(s_{i d})
  + \sum_{t=i d}^{\,i d + d -1}\log P^F
- \log C(s_{(i+1)d})\,R(s_{(i+1)d})
  - \sum_{t=i d}^{\,i d + d -1}\log P^B.
\]
Then the full-trajectory loss can be written as
\begin{align*}
\mathcal{L}^{full}_{hy}
= & ||logC(s_0)R(s_0)+\Sigma_0^{N-1}\log P^F-logC(s_N)R(s_N)-\Sigma_0^{N-1}\log P^B||_2\\
= &\Bigl\|\sum_{i=0}^{\tfrac{N}{d}-1} g_i\Bigr\|_2. 
\end{align*}
By the triangle inequality,
\[
\bigl\|\sum_i g_i\bigr\|_2
\;\le\;
\sum_i \|g_i\|_2.
\]
Since \(E(L^{sub}_{hy})=E(||g_i||_2)=0\), as a result, we have 
$$
0 \le \bigl\|\sum_i g_i\bigr\|_2
\;\le\;
\sum_i \|g_i\|_2=0
$$
This means $\mathcal{L}^{full}_{hy}=0$. Similar to the proof of Theorem~\ref{thm:sub-tra}, we have
\[
E_{\tau\in\mathcal{T}_{0\to N}}\prod_{t=1}^{N-1} P^F_{\phi}(s_{t+1}\mid s_{t}) \;\propto\; R_T(s_N).
\]
\end{proof}
\clearpage

\section{Proofs of Theorem 3}\label{app:prof3}

\begin{lemma}\label{lemma:theta_convergence}
Assume that the loss function \( L_d(\cdot) \) is \( l \)-smooth and satisfies \( \mu \)-strongly convex. Then, the sequence \( \{\theta_{i}\}_{i=0}^{T} \) generated by the gradient descent update with step size \( \frac{1}{l} \) satisfies
\[
\|\theta^{T} - \theta^*\|^2 \leq \frac{2 [L_d(\theta^0) - L_d(\theta^*)]}{\mu} \left(1 - \frac{\mu}{l}\right)^{T}.
\]
\end{lemma}

\begin{proof}
Since \( L_d(\theta) \) is \( l \)-smooth, for any \( \theta \) and \( \theta' \), we have
\begin{equation*}
    L_d(\theta') \leq L_d(\theta) + \nabla L_d(\theta)^\top (\theta' - \theta) + \frac{l}{2} \|\theta' - \theta\|^2.
\end{equation*}

Applying this to the gradient descent update $\theta^{k+1} = \theta^k - \frac{1}{l} \nabla L_d(\theta^k)$, we have
\begin{align}\label{eq:expend}
L_d(\theta^{k+1}) &\leq L_d(\theta^k) + \nabla L_d(\theta^k)^\top (\theta^{k+1} - \theta^k) + \frac{l}{2} \|\theta^{k+1} - \theta^k\|^2 \notag\\
&= L_d(\theta^k) - \frac{1}{2l} \|\nabla L_d(\theta^k)\|^2.
\end{align}

Since  $L_d(\theta)$ is $\mu$-strongly convex, it satisfies the Polyak--Lojasiewicz condition:
\begin{equation*}
\frac{1}{2} \|\nabla L_d(\theta)\|^2 \geq \mu [L_d(\theta) - L_d(\theta^*)].
\end{equation*}

Substituting this inequality into Equation~\ref{eq:expend}, we have
\begin{align*}
L_d(\theta^{k+1}) & \leq L_d(\theta^k) -  \frac{\mu}{l}  (L_d(\theta^k) - L_d(\theta^*)).
\end{align*}

The above equation can be reorganized to
\[
L_d(\theta^{k+1}) - L_d(\theta^*) \leq \left( 1 - \frac{\mu}{l} \right) (L_d(\theta^k) - L_d(\theta^*)).
\]

Start from $k=0$, and recursively apply the above equation $T$ times. It follows that
\[
L_d(\theta^{T}) - L_d(\theta^*) \leq \left( 1 - \frac{\mu}{l} \right)^{T} (L_d(\theta^0) - L_d(\theta^*)).
\]

Since \( L_d(\theta) \) is \( \mu \)-strongly convex, it satisfies
\[
\|\theta - \theta^*\|^2 \leq \frac{2}{\mu} (L_d(\theta) - L_d(\theta^*)).
\]

So we have
\begin{align*}
\|\theta^{T} - \theta^*\|^2 &\leq \frac{2}{\mu} (L_d(\theta^{T}) - L_d(\theta^*)) \\
&\leq \frac{2(L_d(\theta^0) - L_d(\theta^*))}{\mu}  \left( 1 - \frac{\mu}{l} \right)^{T}.
\end{align*}
\end{proof}
\begin{theorem}\label{theorem:emperi error}
When the reconstruction error of the generative model is bounded by \( c \), the downstream loss satisfies \( L_d(\cdot) \leq \psi \), and the loss function is both \( l \)-smooth and \( \mu \)-strongly convex, with the eigenvalues of the Hessian matrix around the optimum \( \theta_* \) bounded by \( \lambda \), the cumulative empirical error of the decoupled weight generation framework can be bounded as follows:
$$
    L_D(\hat{\theta})-L_D(\theta^*) \leq \frac{\lambda}{2} \left[c+\frac{2\psi}{\mu}\left(1 - \frac{\mu}{l}\right)^{T}\right],
$$
where $\hat{\theta}$ is the weight predicted by the generative model.
\end{theorem}
\begin{proof}
Using the Taylor expansion around the optimal point \( \theta^* \), we have
\begin{align}\label{eq:taylor}
L_d(\hat{\theta}) - L_d(\theta^*) &= \nabla L_d(\theta^*)^T (\hat{\theta} - \theta^*) + \frac{1}{2} (\hat{\theta} - \theta^*)^T \nabla^2 L_d(\xi) (\hat{\theta} - \theta^*)\notag\\
&=\frac{1}{2} (\hat{\theta} - \theta^*)^T \nabla^2 L_d(\xi) (\hat{\theta} - \theta^*).
\end{align}

According to a constraint on the Hessian matrix, we have
\begin{equation}\label{eq:hessiam max value}
 \frac{1}{2} (\hat{\theta} - \theta^*)^T \nabla^2 L_d(\xi) (\hat{\theta} - \theta^*) \leq \frac{\lambda}{2}  ||\hat{\theta} - \theta^*||^2.
\end{equation}

Decomposing $|\hat{\theta} - \theta^*||^2$ into weight preparation error and reconstruction error, we have
\begin{align}\label{eq:theta error cumulative}
    ||\hat{\theta}-\theta^*||^2 &\leq ||\hat{\theta}-\theta^{T}||^2 + ||\theta^{T}-\theta^*||^2 \notag\\
&\leq c + \frac{2 \left(L_d(\theta^0) - L_d(\theta^*)\right)}{\mu} \left(1 - \frac{\mu}{l}\right)^{T} \notag (\text{Using Lemma~\ref{lemma:theta_convergence}})\\
& \leq c + \frac{2 \psi}{\mu} \left(1 - \frac{\mu}{l}\right)^{T}.
\end{align}

Substituting Equation~\ref{eq:theta error cumulative} and Equation~\ref{eq:hessiam max value} into Equation~\ref{eq:taylor} we obtain
$$
    L_d(\hat{\theta})-L_d(\theta^*) \leq \frac{\lambda}{2} \left[c+\frac{2\psi}{\mu}\left(1 - \frac{\mu}{l}\right)^{T}\right].
$$
\end{proof}

\clearpage
\section{Experimental Detail}\label{sec:appendix_Experimental Detail}
\subsection{Dataset}\label{sec:dataset setup}
\noindent\textbf{Omniglot.}
The raw Omniglot dataset contains 1623 handwritten characters from 50 alphabets, each with 20 instances in 28$\times$28 grayscale format. We partition the classes of the training set, evaluation set, and testing set into 800:400:432. We use Omniglot in three scenarios. We used the Omniglot dataset in our preliminary experiments, ablation experiments, and comparative experiments. For the construction of the classification task, we referred to the experimental setup by MAML.
\\
\par
\noindent\textbf{Mini-Imagenet.}
The raw Mini-Imagenet contains 100 classes, each containing 600 instances in 84$\times$84 grayscale format. We partition classes of training set, evaluation set, and testing set into 64:16:20. The usage of Mini-Imagenet is the same as Omniglot, and we also follow the setup given by MAML.
\\
\par
\noindent\textbf{Tiered-Imagenet.}
The Tiered-Imagenet dataset is a larger-scale few-shot learning benchmark derived from ImageNet, containing 608 classes grouped into 34 higher-level categories. Each image is in 84$\times$84 resolution with RGB channels. Following the standard protocol (Meta-Baseline), we partition the dataset into 351 classes for training, 97 for validation, and 160 for testing, ensuring no class overlap across phases. We use Tiered-Imagenet in all experimental stages, including ablation and comparative evaluations, to assess the generalization ability of our method on a more diverse and semantically structured dataset.
\\
\par
\noindent\textbf{Imagenet-1K.}
The raw ImageNet-1K is a benchmark dataset with 1000 classes, 1.2 million training images, and 50000 validation images, typically resized to a resolution of 224$\times$224 pixels. We partitioned the dataset into 20k subsets, each containing 50 classes with 50 images per class. We use this dataset for pre-training and perform transfer learning evaluation on other unseen datasets.
\\
\par
\noindent\textbf{CIFAR-10 CIFAR-100 STL-10 Aircraft Pets.}
CIFAR-10 and CIFAR-100 are image datasets introduced by Alex Krizhevsky, containing 60000 images resized to 32$\times$32 pixels. CIFAR-10 includes 10 classes, while CIFAR-100 features 100 fine-grained classes. STL-10, derived from ImageNet, consists of 10 classes with 13000 labeled images and 100000 unlabeled images, with a resolution of 96$\times$96 pixels. The Aircraft dataset includes 10000 images across 100 aircraft models, with hierarchical labels for manufacturer, family, and variant. The Pets dataset consists of 7349 images of 37 pet breeds, with annotations for class labels, bounding boxes, and pixel-level segmentation. We use these datasets to evaluate the model's transfer learning capabilities, which means the labels of these datasets are not visible to the model.
\\
\par
\noindent\textbf{DomainNet.}
DomainNet is a dataset for multi-domain generalization. We use it to evaluate algorithms' ability of few-shot domain generalization. It consists of 345 classes from 6 domains, with a resolution of 224$\times$224 pixels. We use Clipart, Infograph, Painting, Quickdraw, and Real domains for training, while Sketch domains are for testing. The tasks we constructed are 5-way 1-shot and 20-way 5-shot. Note that the testing set shares the same 345 classes as the training set.
\\
\par
\noindent\textbf{GLUE.}
The GLUE Benchmark (General Language Understanding Evaluation) tests models on 9 diverse NLP tasks, including CoLA for grammatical acceptability, SST-2 for sentiment classification, MRPC for paraphrase detection, STS-B for sentence similarity, QQP for duplicate question detection, MNLI for natural language inference, QNLI for question-answer validation, RTE for entailment classification, and WNLI for pronoun resolution. We use this dataset to test the efficiency of different algorithms for multi-task fine-tuning on LLM models. Specifically, we use five binary classification tasks, \ie, SST-2, QQP, RTE, WNIL, and CoLA for the training of \ourmethod. Then we use the other two tasks, \ie, MRPC and QNIL, to evaluate the performance of different fine-tuning algorithms.

\subsection{Model Configuration}
In transfer learning tasks, the downstream network uses ResNet12 with a linear probe for classification. For the generative model $f^G_{\phi}$, \ourmethod employs the same U-Net architecture given by Meta-Diff. In the weight preparation stage, the real optimizers, \ie, SGD and Adam, use a fixed learning rate of 0.005 and an automatic early-stopping strategy to determine the downstream task training epoch $T$. In the policy learning stage, we set the learning rate $\alpha$ and training epochs to 0.001 and 6000, respectively. The acceleration coefficient $k$ is set to 2, and the inference step $N$ is computed as $N=T/k$ for each task. \textbf{We maintain this setup across all experiments in this paper.} In few-shot tasks, following the setting given by MAML, the downstream neural network uses four convolution blocks with a linear probe for classification. In domain generalization tasks, the downstream network uses ResNet12 with a linear probe for classification. In LLM fine-tuning tasks, the large language model we fine-tuned is RoBERTa-base, and the LoRA matrices are generated following the fine-tuning process given by FourierFT.

\subsection{Implementation}
Readers may be concerned about the storage overhead of \ourmethod, as the weight preparation stage appears to require storing a large number of model weights. However, in the implementation, this issue can be avoided through pre-sampling. Specifically, as shown in line 8 of Algorithm 1, the offline trajectory $\tau^{0:T}_{off}$ is sampled in advance. Moreover, as indicated in Equation 7, only the endpoints $\theta_m$ and $\theta_n$ of each sampled offline sub-trajectory $\tau^{m:n}_{off}$ are actually used. Therefore, the storage cost per sampling is $O(1)$. The total storage overhead is thus $O(B)$, where $B$ is the total number of samples, which also corresponds to the number of training steps for the generative model $f^G_{\phi}$.
